# Supplementary material for: Secure Control Systems for Autonomous Quadrotors against Cyber-Attacks
Source: arXiv:2409.11897 source file (2024-09-18)
Supplement: Supplementary file 1 [file appendix1.tex]

\chapter{Comprehensive assembling of an Agilicious quadrotor}
As part of our study, we provide a comprehensive explanation on the setup of an Agilicious system. That is to enhance the documentation provided by the authors, which may be limited in some specific situations, such as when your configuration slightly differs from theirs. Therefore, we provide a detailed approach to setup such a system, compatible with most of the available configurations.

\section{Component list}
The list of components we have used throughout our setup are given below. However, note that most available configurations should be compatible with our guide.
\begin{itemize}
    \item Main Compute Unit: Nvidia Jetson Xavier NX
    \item Breakout board: A203 Carrier board for Jetson Nano/Xavier NX V2
    \item Flight Controller: SpeedyBee F7 V3 FC
    \item Electronic Speed Controller: SpeedyBee BL32 50A 4-in-1 ESC
    \item Radio Receiver: FS-X6B
    \item Radio Transmitter: FS-16X
    \item Main Plate: ?
    \item Motors: ?
    \item Propellers: ?
    \item Battery: Tattu R-Line V3.0 2000mAh 4S 120C LiPo Battery
\end{itemize}

\section{Firmware list}
To follow our recommended process, you will need the following firmware:
\begin{itemize}
    \item A Base Computer running Ubuntu 20.04, with installed: Motive (Mocap software), BetaFlight (FC software - we recommend using a stable release), and ROS.
    \item A On-board (or BaBee) computer running Ubuntu 20.04, with installed: ROS.
\end{itemize}

\section{Mechanical assembling}
The mechanical assembly of the quadrotor’s frame (SpeedyBee Frame V2) can be done following this tutorial: \nolinkurl{https://youtu.be/hWUoH5cyySo?si=n4RCJ04sYB27ETVS}.

\section{Flight Controller (FC) Electronic Assembly}
The electronic assembly of the flight controller (SV-F7V3-BL32-50A) can be done following the tutorials below:
\begin{itemize}
    \item \nolinkurl{https://youtu.be/VfNlDSZoTvc?si=3v8P6FFKEZn0rWTS}
    \item \nolinkurl{https://youtu.be/lw5rZoBxtzk?si=9PThKLTMh40VmC07}
    \item \nolinkurl{https://youtu.be/UVIMAifJjvE?si=jcgfB9_tG2y0-G_0}
\end{itemize}

\section{(Optional) Betfalight Software General Tutorials}
For those unused to Betaflight, we recommend watching the following playlist/serie of videos, which explain in detail every aspect of the software and its configurations: \nolinkurl{https://youtube.com/playlistlist=PLwoDb7WF6c8nT4jjsE4VENEmwu9x8zDiE&si=eUgScTlpqcQ8FIik}.

\section{Flashing Jetson Xavier NX}
In order to flash Jetson Xavier NX on an A203 Carrier Board, you may want to follow the official instructions from the following link: \nolinkurl{https://wiki.seeedstudio.com/reComputer_A203_Flash_System/#flashing-jetpack-osvia-command-line.} \\

Note: We highly recommend not to flash using Nvidia’s SDK Manager. Instead, we suggest using the command line installation steps from the above link. \\

Jetson Linux Version: “35.5.0 $>$”

JetPack version: “5.0.2”

\textbf{TO FINISH LATER}
